# Supplementary material for: Off-Policy Risk Assessment in Markov Decision Processes
Source: arXiv:2209.10444 source file (2022-09-21)
Supplement: Supplementary file 1 [file 4-risk.tex]

\section{Proofs for Risk Estimation (Section~\ref{sec:risk})}
\subsection{Risk Bias and Variance}
% \begin{proof}[Proof of Proposition~\ref{prop:rho_bias_var}]
%     Note that the CDF $F \in \mathcal{L}_\infty (\mathbb{R}, \mathbb{B}(\mathbb{R}))$
%     and risk functional $\rho:\mathcal{L}_\infty (\mathbb{R}, \mathbb{B}(\mathbb{R})) \rightarrow \mathbb{R}$. 
%     If the Frechet derivative of $\rho$ exists with respect to $F$ in the $\mathcal{L}_\infty$ space, then we have the Taylor expansion 

%     \begin{align*}
%         \E\lb \rho(\wh{F}) \rb &= \E\lb \rho\lp F + (\wh{F} - F)\rp  \rb \\ 
%         &\approx \rho(F) + \E\lb D\rho(F)\wh{h}+ \frac{1}{2}\langle D^2\rho(F), \wh{h}\rangle \wh{h} \rb\\ 
%         &= \rho(F) + \frac{1}{2}\E\lb (D\rho(F)\wh{h})^2 \rb \\
%         &=\rho(F) + \frac{1}{2}\E\lb \langle D\rho(F)\otimes D\rho(F),\wh{h}\rangle\wh{h} \rb
%     \end{align*}
%     where $\wh{h} = \wh{F} - F$, $D^k \rho(F)$ denotes the $k$th Frechet derivative of $\rho$ at $F$ and is a multilinear map from $\mathcal{L}_\infty \rightarrow \mathbb{R}$, $\otimes$ denote operator outer product, and $\cdot \wh{h}^k$ means to evaluate a multilinear map at $(\wh{h},\ldots, \wh{h})$. 
    
%     Similarly, 
%     \begin{align*}
%         \Var\lb \rho(\wh{F})\rb &= \Var\lb \rho\lp F + (\wh{F} - F)\rp  \rb \\ 
%         %%
%         &\approx \Var\lb D\rho(F)\wh{h}+ \frac{1}{2}\langle D^2\rho(F), \wh{h}\rangle \wh{h} \rb \\
%         %%
%         &\approx \E\lb \wh{h} \nabla_F\rho \otimes \nabla_F\rho~\wh{h}\rb 
%     \end{align*} 
    
% \end{proof}

\begin{proof}[Proof of Proposition~\ref{prop:rho_bias_var}]
    Note that the CDF $F \in \mathcal{L}_\infty (\mathbb{R}, \mathbb{B}(\mathbb{R}))$
    and risk functional $\rho:\mathcal{L}_\infty (\mathbb{R}, \mathbb{B}(\mathbb{R})) \rightarrow \mathbb{R}$. 
    If the Fr\'echet derivative of $\rho$ exists with respect to $F$ in the $\mathcal{L}_\infty$ space, then using the Taylor expansion, we have,

    \begin{align*}
        \E\lb \rho(\wh{F}) \rb &= \E\lb \rho\lp F + (\wh{F} - F)\rp  \rb \\ 
        &\approx \rho(F) + \E\lb \langle\nabla_F \rho,\wh{h}\rangle+ \frac{1}{2}\langle\wh{h}\langle \nabla_F^2\rho, \wh{h}\rangle\rangle  \rb \\
        &= \rho(F) + \frac{1}{2}\E\lb \langle\wh{h}\langle\nabla_F^2\rho, \wh{h}\rangle\rangle  \rb \\
        &\leq \rho(F) + \frac{\|\nabla_F^2\rho\|}{2}\E\lb \langle\wh{h}, \wh{h}\rangle  \rb \\
        % &= \rho(F) + \frac{1}{2} \E\lb\langle D^2 \rho(F), \langle \wh{h}, \wh{h} \rangle \rangle\rb
    \end{align*}
    where $\wh{h} = \wh{F} - F$, and the orders of Fr\'echet derivatives are maps to $\mathbb{R}$ with proper interproducts. Let $\otimes$ denote operator outer product, then we have,

    \begin{align*}
        \Var\lb \rho(\wh{F})\rb &= \Var\lb \rho\lp F + (\wh{F} - F)\rp  \rb \\ 
        &\approx \Var\lb \nabla_F\rho\wh{h}+ \frac{1}{2}\langle \nabla_F^2\rho, \wh{h}\rangle \wh{h} \rb \\
        &\approx \E\lb \wh{h} \nabla_F\rho \otimes \nabla_F\rho~\wh{h}\rb \\
        &\leq ||\nabla_F \rho \otimes \nabla_F \rho||_{op} \E[\langle \wh{h}, \wh{h} \rangle]
    \end{align*} 
  
  $$
  \mathbb{E}[(\int_0^D \wh F(t) - F(t) dt)^2]
  = \mathbb{E}[(\int_0^D \wh F(t) - 1 dt + \int_0^D  1- F(t) dt)^2]
  = \mathbb{E}[(\text{empirical mean} - \text{true mean})^2]
  = \text{Var}(\text{empirical mean})
  $$  
    
\end{proof}
$U,V$ is defined in $L_\infty(\mu, \mathcal{D})$, $W$ is defined on $L_2(\mu, \R)$. 

Here $\rho : U \rightarrow W$, and 
$\nabla_F \rho : V \rightarrow W$. Also $F \in U$ and $h \in V$. 

$$ ||\nabla_F \rho \otimes \nabla_F \rho||_{op} = \sup_h \frac{||\nabla_F \rho \otimes \nabla_F \rho h ||_\infty}{||h||_\infty} =  \sup _h \frac{||\nabla_F \rho||_\infty \cdot |\nabla_F \rho h|}{||h||_\infty}  = \sup_{g,h} \frac{|\int_\D g(x)dx| \cdot |\int_\D h(x)dx|}{||g||_\infty||h||_\infty} $$

% https://www.cs.cmu.edu/~epxing/Class/10708-14/lectures/lecture22-HSEmbedding.pdf

\begin{proof}[Proof of Corollary~\ref{cor:lipschitz_error}]
    The bound is a direct application of the definition of Lipschitz risks (Definition~\ref{cor:lipschitz_error}) and the error bounds for off-policy CDF estimates (e.g. Lemma~\ref{lem:is_error}). 
\end{proof}

\input{appendix/4.1-risk_lower_bound}
